# Supplementary material for: Fast exploration of chemical reaction networks
Source: arXiv:1405.6610 source file (2014-05-26)
Supplement: Supplementary file 1 [file supmat.pdf]

This document contains additional details on the computational procedure employed in the examples of the fast network exploration method presented in the main paper.

The molecular dynamics simulations were performed by employing LAMMPS code [1] compiled with the PLUMED [2] plugin (version 1.3) that was modified to use the potential energy as collective variable.

## SINGLE ATOM IN 2D POTENTIAL

The two dimensional model system evolved in a potential described by the following equation:

$$U(x, y) = a_x x^6 + 7a_x x^4 + 12a_x x^2 + d_x x + a_y y^2 \tag{1}$$

Initial tests were performed on symmetric systems ($d_x = 0$) without (Tab. I) and with (Tab. II) a thermostat. The height $h_H$ and width $\sigma_H$ of the Gaussian shaped bias (both listed below in kcal/mol) as well as the rate of bias deposition $\delta_H$ (in ps) were varied. Both well-tempered Metadynamics, with different values of the bias factor BF and "plain" Metadynamics (BF $= \infty$) were employed. For each system the average and standard deviation of temperature ($\langle T \rangle$ and $\sigma_T$ both in K) and simulation time ($\langle t \rangle$ and $\sigma_t$ in ps) are reported.

A second set of tests was performed with asymmetric potentials, again without (Tab. III) and with (Tab. IV) the presence of a thermostat. As in the previous case, the application of a thermostat is expected not to affect the ratio between the rates due to the lack of vibrational degrees of freedom of the system. The $\Delta G^{\ddagger}$ needed to compute the theoretical ratio was evaluated from Eq. 1, since there is no relevant difference in the entropic contribution of the two pathways.

## ETHANE

Ethane simulations were performed with a time-step of 0.1 fs. The theoretical rates were computed by extrapolating the FE for the C−H and C−C bond breaking at the system temperature. To do that the FE of both reactions was computed at 500, 1000, 1500 and 2000 K (see Fig. 1), by using well-tempered Metadynamics and the relevant bond distance as a collective variable. The data reported in Fig. 1 is the FE difference between the bonded

and the transition state. The former is defined as the region around the minimum MIN that has an energy up to $2k_BT$ more than MIN, while the latter is the region around the maximum that has an energy up to $\frac{1}{2}k_BT$ less than the barrier.

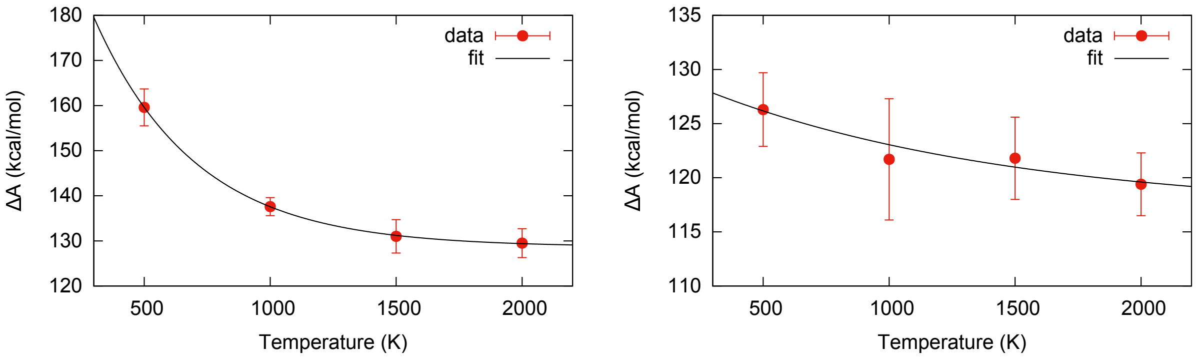


(a) C-C bond breaking

(b) C-H bond breaking

FIG. 1: Computed FE for the C-C and C-H bond breaking for the ethane molecule at different temperatures shown with the 95% confidence interval. The black lines show the exponential fitting.

The comparison for different simulations settings are listed in Tab. V, where we have tested the consistency of the results for different biasing parameters.

## DECALIN

Decalin simulations followed the same general protocol used for ethane, with the addition of a soft wall placed on the distance between the center of mass of the methyl and the decalin molecules at 0.8 nm. Results are reported in Tab. VI. The theoretical FE for the reactions were separated in 4 groups: the C−H bond breaking (reactions 1, 2, and 3), the C−C bond breaking (reactions 4, 5, 7, and 8), the isomerization (reaction 6) and the hydrogen abstractions (reactions 1a, 2a, and 3a). For the first two groups, as shown in Fig. 2, the differences between each single reactions are in general smaller than the accuracy of the (fe) calculations therefore they were used together to build a general fitting function by computing (fe) for each of them at different temperatures (500, 700, 800, 1000, 1500 and 2000 K). To obtain these values the well-tempered Metadynamics algorithm was used, biasing the relevant bond distance.

Hydrogen abstractions reactions by the methyl radical were instead studied by simultaneously biasing the specific C−H bond and the distance between the hydrogen and the methyl radical carbon. As illustrated by Fig. 3 the presence of the methyl radical does not facilitate the C−H bond breaking.

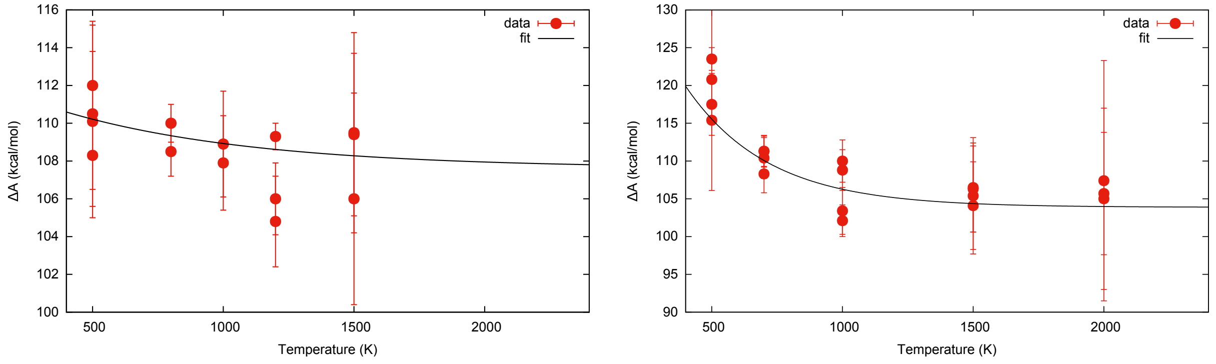


(a) C-C bond breaking (b) C-H bond breaking

FIG. 2: Computed FE for the C-C and C-H bond breaking for the *t*-decalin molecule at different temperatures reported with the 95% confidence interval. The black lines show the exponential fitting.

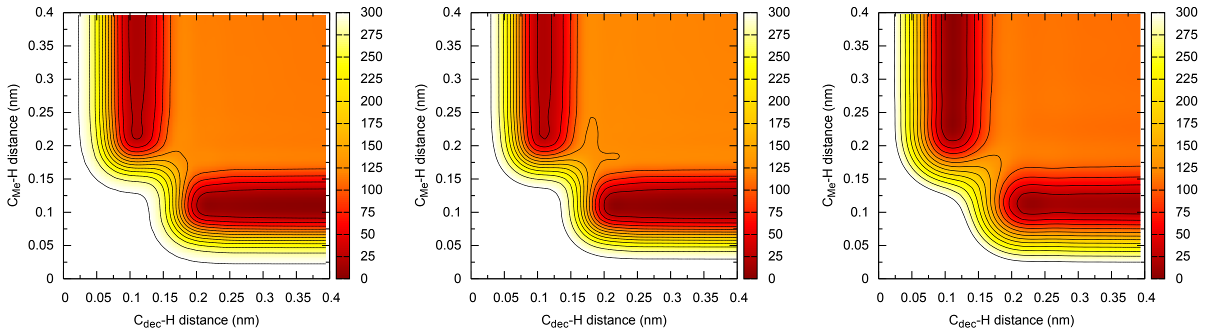


(a) Reaction 1a (b) Reaction 2a (c) Reaction 3a

FIG. 3: Free energy projections for the three possible decalin hydrogen abstractions by a methyl radical. Energy is reported in kcal/mol and isolines are drawn every 25 kcal/mol.


[1] S. Plimpton, Journal of Computational Physics **117**, 119 (1995).

[2] M. Bonomi, D. Branduardi, G. Bussi, C. Camilloni, D. Provasi, P. Raiteri, D. Donadio, F. Marinelli, F. Pietrucci, R. A. Broglia, and M. Parrinello, Computer Physics Communications **180**, 1961 (2009).

TABLE I: Results for different symmetric two dimensional potentials systems simulated without a thermostat. Bias shape parameters ($h_H$, $\sigma_H$) as well as free energy barriers ($\Delta G^{\ddagger}_{CC}$, $\Delta G^{\ddagger}_{CH}$) are listed in kcal/mol, while bias addition frequency $\delta_H$ is expressed in ps; masses are reported in Dalton. Temperature average and standard deviation ($\langle T \rangle$, $\sigma_T$) are expressed in K; time average and standard deviation ($\langle t \rangle$, $\sigma_t$) are in ps. The "Neg." and "Pos." columns refer to the number of observed simulations ending in the negative ($x < -1$) or positive ($x > 1$) basins, respectively.

| BF | $h_H$ | $\sigma_H$ | $\delta_H$ | $a_x$ | $a_y$ | Runs | $\langle T \rangle$ | $\sigma_T$ | $\langle t \rangle$ | $\sigma_t$ | Neg. | Pos. |
|---|---|---|---|---|---|---|---|---|---|---|---|---|
| 3 | 0.05 | 0.05 | 1 | 4 | 2 | 60 | 1286 | 466 | 2.39 | 2.78 | 32 | 28 |
| 3 | 0.05 | 0.05 | 1 | 4 | 4 | 60 | 1341 | 541 | 1.91 | 1.93 | 27 | 33 |
| $\infty$ | 0.05 | 0.05 | 1 | 2 | 2 | 60 | 639 | 300 | 2.19 | 2.05 | 31 | 29 |
| 3 | 0.05 | 0.05 | 1 | 2 | 2 | 60 | 570 | 246 | 2.77 | 2.89 | 32 | 28 |
| 3 | 0.01 | 0.01 | 1 | 2 | 2 | 60 | 1017 | 843 | 2.08 | 1.87 | 28 | 32 |
| 3 | 0.01 | 0.01 | 0.1 | 2 | 2 | 60 | 1004 | 288 | 1.01 | 1.31 | 35 | 25 |
| 3 | 0.01 | 0.01 | 0.05 | 2 | 2 | 60 | 965 | 336 | 0.74 | 0.69 | 29 | 31 |
| 3 | 0.1 | 0.1 | 10 | 2 | 2 | 60 | 301 | 112 | 24.10 | 22.55 | 25 | 35 |
| 3 | 0.01 | 0.03 | 0.05 | 2 | 2 | 60 | 867 | 255 | 1.58 | 1.38 | 34 | 26 |
| 3 | 0.01 | 0.1 | 0.05 | 2 | 2 | 60 | 403 | 155 | 10.63 | 4.82 | 26 | 34 |
| 3 | 0.01 | 0.1 | 0.05 | 10 | 10 | 160 | 3507 | 1113 | 2.36 | 1.90 | 83 | 77 |
| 10 | 0.01 | 0.1 | 0.05 | 10 | 10 | 160 | 3823 | 1372 | 2.70 | 2.28 | 79 | 81 |
| 25 | 0.01 | 0.1 | 0.05 | 10 | 10 | 160 | 3980 | 1264 | 1.65 | 2.26 | 89 | 71 |
| 50 | 0.01 | 0.1 | 0.05 | 10 | 10 | 160 | 3724 | 1203 | 1.90 | 2.28 | 90 | 70 |
| 100 | 0.01 | 0.1 | 0.05 | 10 | 10 | 160 | 3904 | 1392 | 1.80 | 2.12 | 86 | 74 |
| 10 | 0.01 | 0.1 | 0.05 | 3 | 3 | 100 | 1250 | 420 | 2.17 | 2.34 | 47 | 53 |
| 10 | 0.01 | 0.1 | 0.05 | 10 | 2 | 100 | 3587 | 1237 | 2.09 | 2.61 | 58 | 42 |

TABLE II: Results for different symmetric two dimensional potentials systems simulated with a thermostat. Bias shape parameters ($h_H$, $\sigma_H$) as well as free energy barriers ($\Delta G^{\ddagger}_{CC}$, $\Delta G^{\ddagger}_{CH}$) are expressed in kcal/mol, while bias addition frequency $\delta_H$ is listed in ps; masses are reported in Dalton. Temperature average and standard deviation ($\langle T \rangle$, $\sigma_T$) are expressed in K; time average and standard deviation ($\langle t \rangle$, $\sigma_t$) are in ps. The "Thermo" column refers to the type of thermostat (Lan for Langevin and NHc10 for a Nose-Hoover chain of lenght 10), applied with a time constant $\tau$ (in ps). The "Neg." and "Pos." columns refer to the number of observed simulations ending in the negative ($x < -1$) or positive ($x > 1$) basins, respectively.

| BF | $h_H$ | $\sigma_H$ | $\delta_H$ | $a_x$ | $a_y$ | Thermo | $\tau$ | Runs | $\langle T \rangle$ | $\sigma_T$ | $\langle t \rangle$ | $\sigma_t$ | Neg. | Pos. |
|---|---|---|---|---|---|---|---|---|---|---|---|---|---|---|
| 3 | 0.05 | 0.05 | 1 | 4 | 2 | Lan | 10 | 60 | 1462 | 427 | 1.95 | 2.72 | 35 | 25 |
| 3 | 0.05 | 0.05 | 1 | 4 | 2 | Lan | 1 | 60 | 1575 | 430 | 1.04 | 0.72 | 34 | 26 |
| 3 | 0.05 | 0.05 | 1 | 4 | 2 | Lan | 0.1 | 58 | 1944 | 644 | 3.86 | 9.48 | 30 | 28 |
| 3 | 0.05 | 0.05 | 1 | 4 | 2 | NHc10 | 10 | 60 | 1518 | 425 | 1.02 | 2.04 | 26 | 34 |
| 3 | 0.05 | 0.05 | 1 | 4 | 2 | NHc10 | 1 | 59 | 1535 | 550 | 1.57 | 6.44 | 26 | 33 |
| 3 | 0.05 | 0.05 | 1 | 4 | 2 | NHc10 | 0.1 | 60 | 1453 | 451 | 7.22 | 12.56 | 31 | 29 |
| 3 | 0.01 | 0.1 | 0.05 | 4 | 2 | NHc10 | 0.1 | 38 | 901 | 128 | 21.30 | 11.61 | 21 | 17 |
| 3 | 0.01 | 0.1 | 0.05 | 4 | 2 | NHc10 | 10 | 100 | 897 | 440 | 4.66 | 3.82 | 45 | 55 |

TABLE III: Results for different asymmetric two dimensional potentials systems simulated without a thermostat. Bias shape parameters ($h_H$, $\sigma_H$) as well as free energy barriers ($\Delta G^{\ddagger}_{CC}$, $\Delta G^{\ddagger}_{CH}$) are expressed in kcal/mol, while bias addition frequency $\delta_H$ is listed in ps; masses are reported in Dalton. Temperature average and standard deviation ($\langle T \rangle$, $\sigma_T$) are expressed in K; time average and standard deviation ($\langle t \rangle$, $\sigma_t$) are in ps. The "Neg." and "Pos." columns refer to the number of observed simulations ending in the negative ($x < -1$) or positive ($x > 1$) basins, respectively.

| BF | $h_H$ | $\sigma_H$ | $\delta_H$ | $a_x$ | $a_y$ | $d_x$ | Runs | $\langle T \rangle$ | $\sigma_T$ | $\langle t \rangle$ | $\sigma_t$ | Neg. | Pos. |
|---|---|---|---|---|---|---|---|---|---|---|---|---|---|
| 3 | 0.01 | 0.1 | 0.05 | 2 | 2 | 1 | 60 | 508 | 193 | 5 | 5 | 59 | 1 |
| 3 | 0.05 | 0.05 | 1 | 4 | 4 | 1 | 60 | 1327 | 392 | 2 | 2 | 56 | 4 |
| 3 | 0.05 | 0.05 | 1 | 3 | 3 | 1.4 | 60 | 940 | 361 | 2 | 2 | 56 | 4 |
| $\infty$ | 0.05 | 0.05 | 1 | 3 | 3 | 1.4 | 60 | 989 | 495 | 2 | 3 | 57 | 3 |
| 3 | 0.05 | 0.05 | 1 | 3 | 3 | 1.4 | 60 | 488 | 286 | 5 | 4 | 58 | 2 |
| 3 | 0.01 | 0.01 | 0.1 | 3 | 3 | 1.4 | 60 | 1164 | 424 | 1 | 2 | 56 | 4 |
| 3 | 0.05 | 0.05 | 1 | 3 | 3 | 1.4 | 60 | 1252 | 297 | 1 | 2 | 59 | 1 |
| 3 | 0.01 | 0.1 | 0.05 | 3 | 3 | 0.6 | 60 | 587 | 328 | 6 | 3 | 55 | 5 |
| 25 | 0.01 | 0.1 | 0.05 | 2 | 2 | 0.6 | 97 | 1227 | 603 | 4 | 8 | 76 | 21 |
| 3 | 0.01 | 0.1 | 0.05 | 2 | 2 | 0.6 | 99 | 747 | 245 | 3 | 3 | 88 | 11 |
| 3 | 0.01 | 0.1 | 0.05 | 10 | 10 | 0.6 | 86 | 1440 | 975 | 7 | 4 | 85 | 1 |

TABLE IV: Results for different symmetric two dimensional potentials systems simulated with a thermostat. Bias shape parameters ($h_H$, $\sigma_H$) as well as free energy barriers ($\Delta G^{\ddagger}_{CC}$, $\Delta G^{\ddagger}_{CH}$) are expressed in kcal/mol, while bias addition frequency $\delta_H$ is listed in ps; masses are reported in Dalton. Temperature average and standard deviation ($\langle T \rangle$, $\sigma_T$) are expressed in K; time average and standard deviation ($\langle t \rangle$, $\sigma_t$) are in ps. "Thermo" column refers to the type of thermostat (Lan for Langevin and NHc10 for a Nose-Hoover chain of length 10), applied with a time constant $\tau$ (in ps). "Neg." and "Pos." columns refer to the number of observed simulations ending in the negative ($x < -1$) or positive ($x > 1$) basins, respectively.

| BF | $h_H$ | $\sigma_H$ | $\delta_H$ | $a_x$ | $a_y$ | $d_x$ | Thermo | $\tau$ | Runs | $\langle T \rangle$ | $\sigma_T$ | $\langle t \rangle$ | $\sigma_t$ | Neg. | Pos. |
|---|---|---|---|---|---|---|---|---|---|---|---|---|---|---|---|
| 3 | 0.01 | 0.1 | 0.05 | 2 | 2 | 0.6 | NHc10 | 0.01 | 120 | 508 | 19 | 19.87 | 14.24 | 107 | 13 |
| 3 | 0.01 | 0.1 | 0.05 | 2 | 2 | 0.6 | NHc10 | 0.05 | 52 | 567 | 61 | 7.27 | 3.77 | 46 | 6 |
| 3 | 0.01 | 0.1 | 0.05 | 2 | 2 | 0.6 | NHc10 | 0.1 | 98 | 656 | 153 | 7.06 | 10.86 | 86 | 12 |
| 3 | 0.01 | 0.1 | 0.05 | 2 | 2 | 0.6 | NHc10 | 0.05 | 100 | 1389 | 432 | 1.17 | 2.86 | 64 | 36 |
| 1.5 | 0.01 | 0.1 | 0.05 | 2 | 2 | 0.6 | NHc10 | 0.05 | 97 | 1228 | 275 | 3.52 | 3.91 | 74 | 23 |
| 50 | 0.01 | 0.1 | 0.05 | 2 | 2 | 0.6 | NHc10 | 0.05 | 100 | 763 | 215 | 3.29 | 5.67 | 83 | 17 |
| 50 | 0.01 | 0.1 | 0.05 | 8 | 8 | 0.15 | NHc10 | 0.05 | 65 | 1657 | 204 | 17.95 | 5.09 | 47 | 18 |
| 50 | 0.01 | 0.1 | 0.05 | 12 | 12 | 0.1 | NHc10 | 0.05 | 32 | 2580 | 771 | 19.90 | 15.09 | 21 | 11 |

TABLE V: Results for the simulations of the ethane reactivity. Bias shape parameters ($h_H$, $\sigma_H$) as well as free energy barriers ($\Delta G^{\ddagger}_{CC}$, $\Delta G^{\ddagger}_{CH}$) are expressed in kcal/mol, while bias addition frequency $\delta_H$ is listed in ps; masses are reported in Dalton. Temperature average and standard deviation ($\langle T \rangle$, $\sigma_T$) are expressed in K; time average and standard deviation ($\langle t \rangle$, $\sigma_t$) are in ps. The "CC" and "CH" columns refer to the number of observed simulations ending with a C−C or a C−H bond breaking.

| BF | $h_H$ | $\sigma_H$ | $\delta_H$ | $m_C$ | $m_H$ | $\Delta G^{\ddagger}_{CC}$ | $\Delta G^{\ddagger}_{CH}$ | Runs | $\langle T \rangle$ | $\sigma_T$ | $\langle t \rangle$ | $\sigma_t$ | CC | CH |
|---|---|---|---|---|---|---|---|---|---|---|---|---|---|---|
| 3 | 0.01 | 0.1 | 0.05 | 12 | 1 | 129 | 119 | 100 | 2460 | 505 | 7.79 | 2.14 | 2 | 98 |
| ∞ | 0.01 | 0.1 | 0.05 | 12 | 1 | 129 | 118 | 200 | 2887 | 654 | 5.11 | 2.93 | 5 | 195 |
| 3 | 0.1 | 0.25 | 1 | 12 | 1 | 136 | 122 | 39 | 1057 | 374 | 47.10 | 31.65 | 1 | 38 |
| 3 | 0.25 | 0.25 | 1 | 12 | 1 | 129 | 120 | 40 | 2905 | 697 | 3.89 | 2.16 | 1 | 39 |
| 3 | 0.25 | 0.25 | 1 | 12 | 1 | 132 | 121 | 40 | 1417 | 593 | 13.05 | 9.41 | 0 | 40 |
| 3 | 1 | 0.25 | 1 | 12 | 1 | 129 | 120 | 40 | 4134 | 970 | 0.94 | 0.51 | 0 | 40 |
| 3 | 1 | 0.25 | 1 | 12 | 1 | 129 | 120 | 40 | 2738 | 989 | 1.26 | 0.92 | 2 | 38 |
| 3 | 1 | 0.25 | 1 | 12 | 1 | 129 | 120 | 38 | 2632 | 826 | 1.25 | 0.97 | 0 | 38 |
| 3 | 1 | 0.25 | 1 | 12 | 1 | 129 | 120 | 39 | 2760 | 1021 | 1.38 | 0.94 | 0 | 39 |
| 3 | 1 | 0.25 | 1 | 12 | 1 | 132 | 121 | 40 | 1358 | 593 | 2.97 | 1.72 | 1 | 39 |
| 3 | 1 | 0.25 | 1 | 12 | 1 | 132 | 121 | 34 | 1336 | 720 | 2.96 | 1.98 | 0 | 34 |
| 250 | 1 | 0.25 | 1 | 12 | 1 | 129 | 120 | 40 | 3985 | 799 | 0.94 | 0.49 | 0 | 40 |
| 250 | 1 | 0.25 | 1 | 12 | 1 | 129 | 120 | 40 | 2634 | 761 | 1.45 | 0.98 | 1 | 39 |
| 250 | 1 | 0.25 | 1 | 12 | 1 | 129 | 120 | 40 | 2860 | 994 | 1.44 | 1.20 | 1 | 39 |
| 3 | 4 | 0.25 | 1 | 12 | 1 | 133 | 121 | 35 | 1264 | 593 | 0.84 | 0.78 | 1 | 34 |
| ∞ | 0.01 | 0.1 | 0.05 | 12 | 2 | 129 | 119 | 197 | 2412 | 682 | 8.70 | 4.22 | 7 | 190 |
| ∞ | 0.01 | 0.1 | 0.05 | 12 | 3 | 129 | 119 | 197 | 2124 | 663 | 11.80 | 7.74 | 5 | 192 |
| 3 | 0.01 | 0.1 | 0.05 | 12 | 4 | 131 | 121 | 70 | 1586 | 567 | 23.60 | 10.09 | 4 | 66 |
| ∞ | 0.01 | 0.1 | 0.05 | 12 | 4 | 129 | 119 | 194 | 2102 | 626 | 14.70 | 10.86 | 4 | 190 |
| 3 | 1 | 0.25 | 1 | 12 | 4 | 129 | 120 | 40 | 2204 | 646 | 5.32 | 2.86 | 0 | 40 |
| 3 | 1 | 0.25 | 1 | 12 | 4 | 147 | 124 | 29 | 722 | 176 | 102.89 | 68.14 | 2 | 27 |
| ∞ | 0.01 | 0.1 | 0.05 | 12 | 5 | 130 | 120 | 182 | 1848 | 607 | 17.52 | 10.75 | 5 | 177 |
| ∞ | 0.01 | 0.1 | 0.05 | 12 | 9 | 131 | 121 | 91 | 1551 | 486 | 35.28 | 15.10 | 2 | 89 |
| 3 | 1 | 0.25 | 1 | 12 | 9 | 148 | 124 | 11 | 701 | 165 | 171.73 | 55.19 | 0 | 11 |

TABLE VI: Results for the simulations of the $t$-decalin reactivity. In both cases Metadynamics algorithm was used (BF = $\infty$), with $\sigma_H = 0.1$ kcal/mol and $\delta_H = 0.1$ kcal/mol. Temperature average and standard deviation ($\langle T \rangle$, $\sigma_T$) are listed in K; time average and standard deviation ($\langle t \rangle$, $\sigma_t$) are in ps. Reactions are marked according to the labels defined in the main text.

| | | | | | | Occurrences | | | | | | | | $\Delta G^{\ddagger}$ (kcal/mol) | | | | | | | |
|---|---|---|---|---|---|---|---|---|---|---|---|---|---|---|---|---|---|---|---|---|---|
| $\delta_H$ | Runs | $\langle T \rangle$ | $\sigma_T$ | $\langle t \rangle$ | $\sigma_t$ | 1 | 2 | 3 | 4 | 5 | 6 | 7 | 8 | 1 | 2 | 3 | 4 | 5 | 6 | 7 | 8 |
| 0.05 | 181 | 2424 | 435 | 11.52 | 7.20 | 62 | 59 | 10 | 7 | 20 | 1 | 18 | 4 | 104 | 104 | 104 | 108 | 108 | 115 | 108 | 108 |
| 0.01 | 183 | 2246 | 931 | 7.40 | 7.08 | 64 | 61 | 14 | 6 | 14 | 3 | 11 | 10 | 104 | 104 | 104 | 108 | 108 | 115 | 108 | 108 |
